# Supplementary material for: Data-Efficient 3D Visual Grounding via Order-Aware Referring
Source: arXiv:2403.16539 source file (2025-02-23)
Supplement: Supplementary file 1 [file overview.tex]

\setcounter{page}{1}
This is the supplementary material of our main manuscript, which includes detailed algorithms of our training method, implementation details of our framework, and more quantitative/qualitative results. Specifically, in \ref{sup:algorithm}, we present the pseudo code for order-aware pre-training sample synthesis and DOrA's complete training pipeline. In \ref{sup:implementation details}, we elaborate on the implementation details of our proposed DOrA and the baselines. In \ref{sup:prompts}, we display the complete prompts for our two-stage ICL, with some examples provided and output results of CoT3DRef's~\cite{bakr2023cot3dref} prompts being the baseline. In \ref{sup:loss ablation}, we conduct the ablation study on proposed losses that help establish the awareness of referential order and identity of anchor objects. In \ref{sup:order length as subsets}, we investigate DorA's performance on samples with different order lengths. Finally, in \ref{sup:more visualization}, we demonstrate the visualization of object features in DOrA's different Object-Referring blocks.
